# Supplementary material for: CVF-SID: Cyclic multi-Variate Function for Self-Supervised Image Denoising by Disentangling Noise from Image
Source: arXiv:2203.13009 source file (2022-03-29)

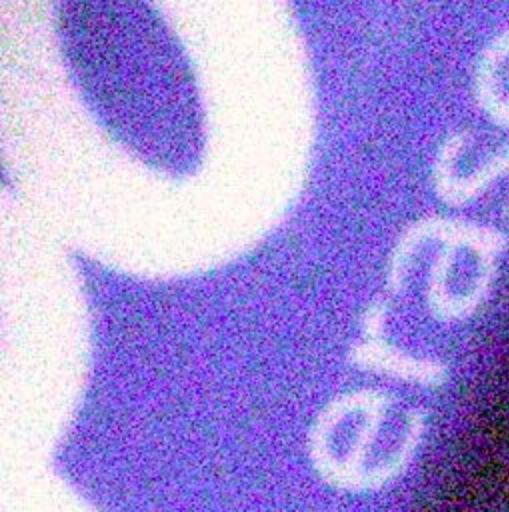







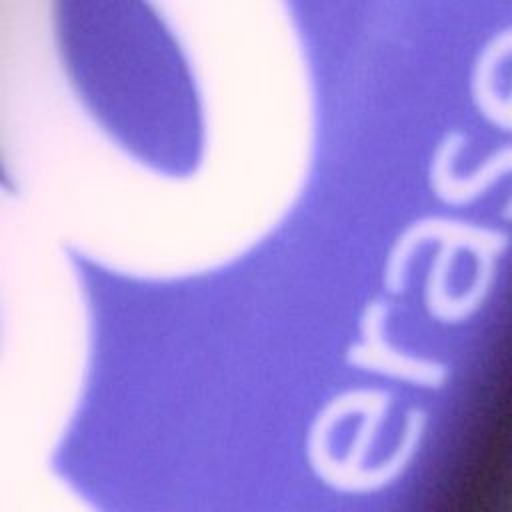

Supplement: Supplementary file 5 [file supp_316.pdf]
