# Supplementary material for: CVF-SID: Cyclic multi-Variate Function for Self-Supervised Image Denoising by Disentangling Noise from Image
Source: arXiv:2203.13009 source file (2022-03-29)

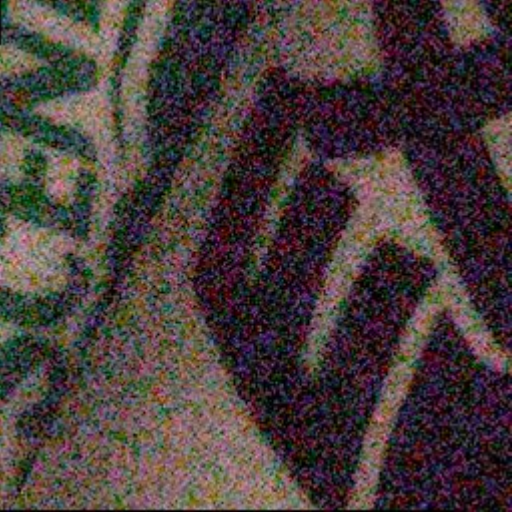

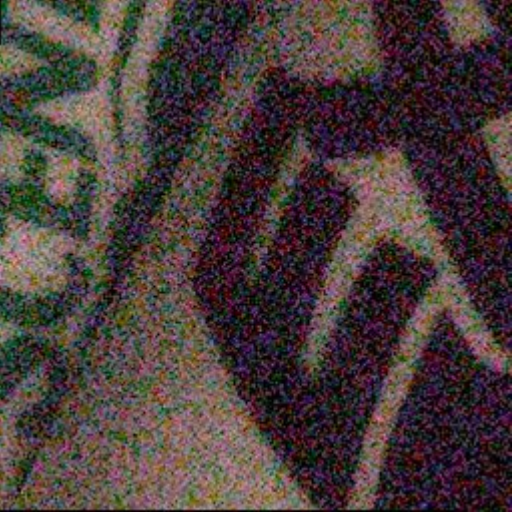

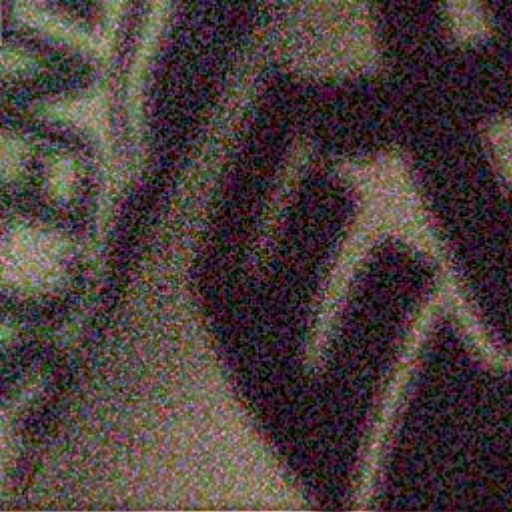



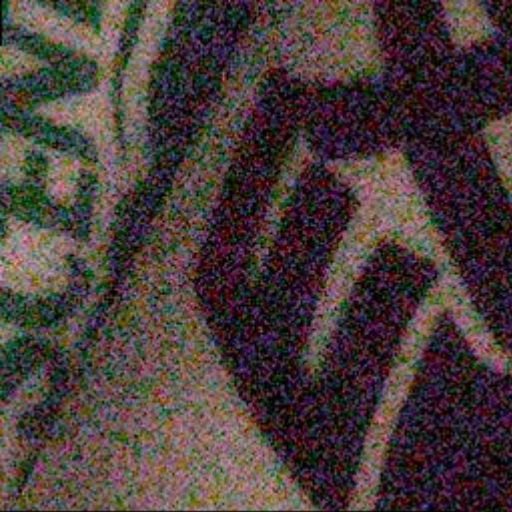

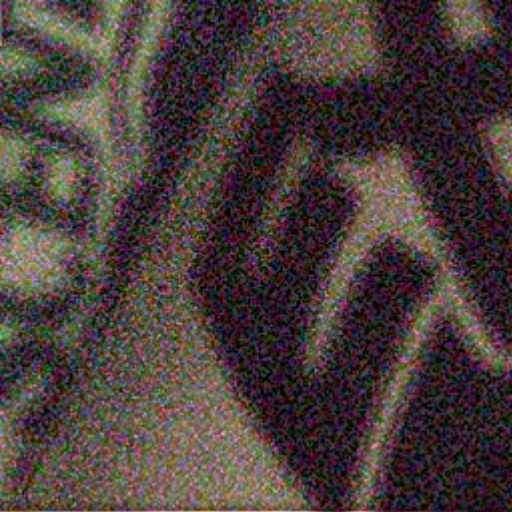

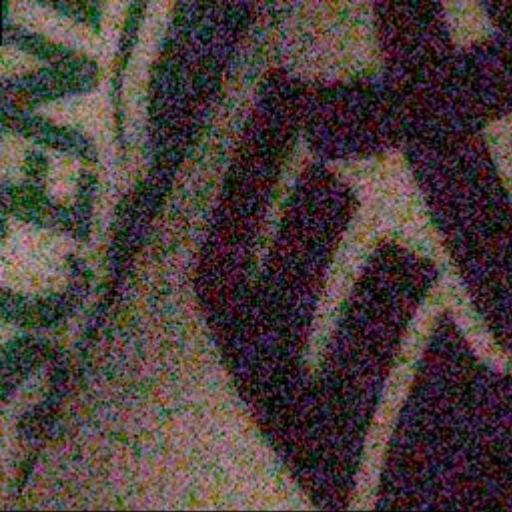

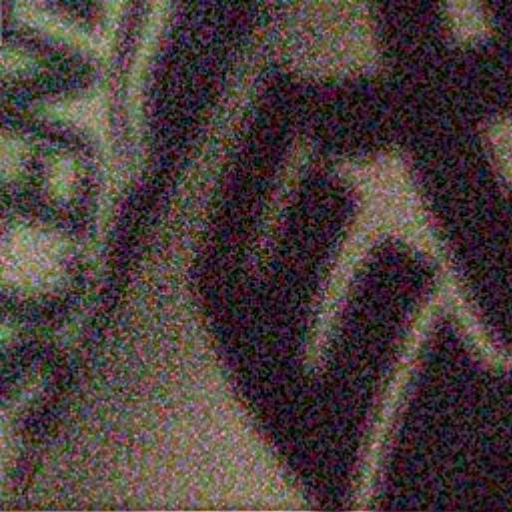

Supplement: Supplementary file 10 [file supp_aug_182.pdf]
