# Supplementary material for: CVF-SID: Cyclic multi-Variate Function for Self-Supervised Image Denoising by Disentangling Noise from Image
Source: arXiv:2203.13009 source file (2022-03-29)

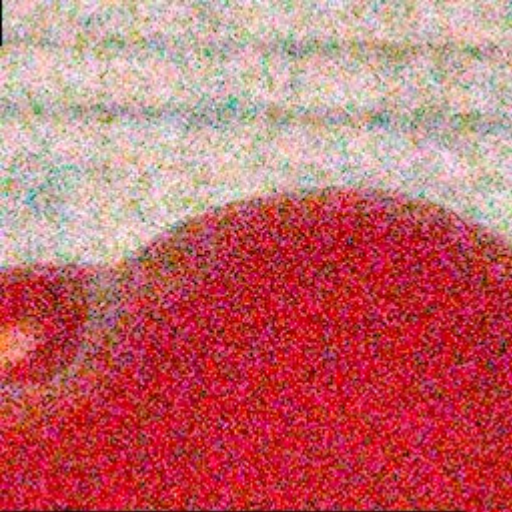

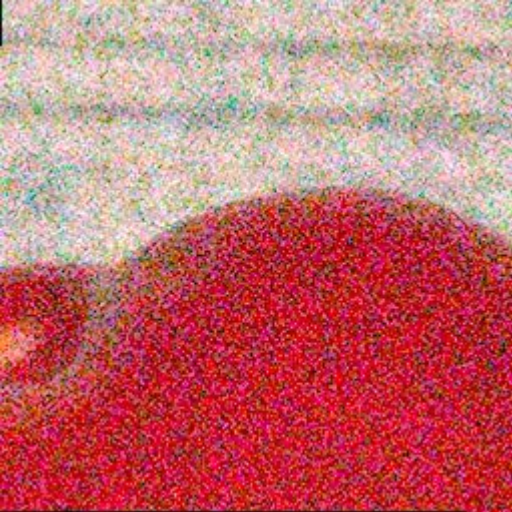

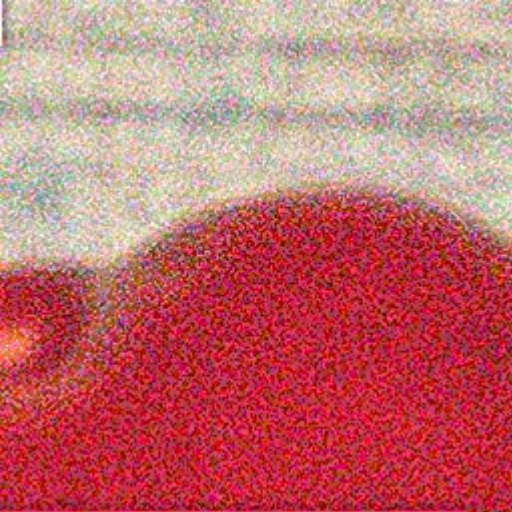



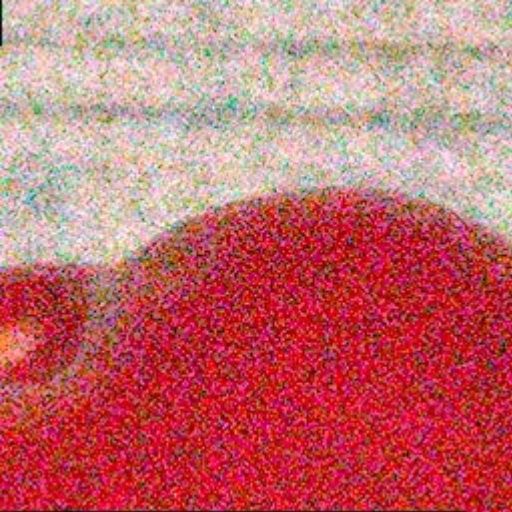

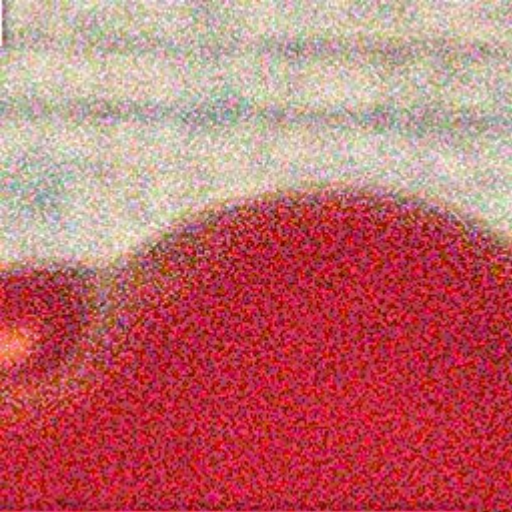

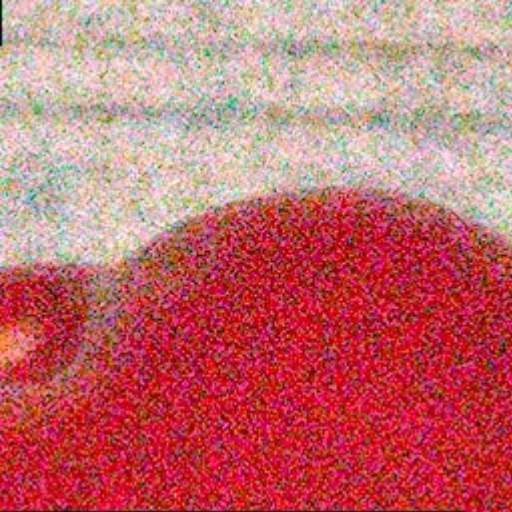

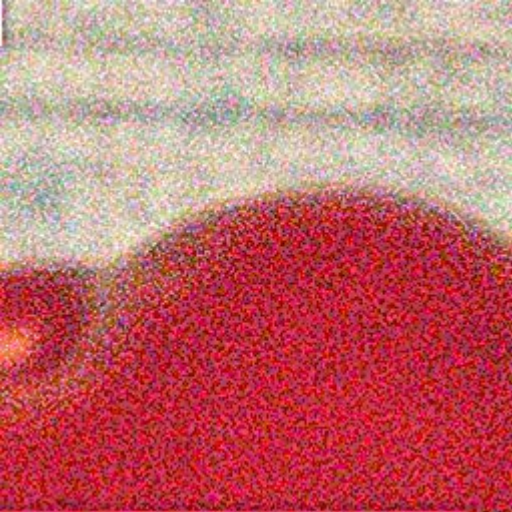

Supplement: Supplementary file 13 [file supp_aug_736.pdf]
